# Supplementary material for: Fano Resonance in an Electrically Driven Plasmonic Device
Source: arXiv:1601.00315 source file (2016-01-03)
Supplement: Supplementary file 1 [file Supplementary_2.pdf]

# Supporting Information

## Fano Resonance in an Electrically Driven Plasmonic Device

*Yuval Vardi*, Eyal Cohen-Hoshen, Guy Shalem and Israel Bar-Joseph*

*Department of Condensed Matter Physics, Weizmann Institute of Science, Rehovot 76100, Israel*

**E-mail: yuval.vardi@weizmann.ac.il*

## Contents

S1 Methods ..... 2
S1.1 Gold nanoparticles synthesis ..... 2
S1.1.1 13 nm Gold NP Synthesis ..... 2
S1.1.2 30 nm Gold NP Synthesis ..... 2
S1.1.3 55 nm Gold NP Synthesis ..... 2
S1.2 Device fabrication and electrostatic trapping ..... 3
S2 Single dot simulation ..... 5
S2.1 Fit parameters ..... 6
S3 Symmetric and Asymmetric devices ..... 7
S4 Extraction of plasmonic spectrum lineshape from total intensity measurement ..... 8
S5 FDTD Simulation ..... 9
S5.1 FDTD details ..... 9
S5.2 Insensitivity to electrodes design ..... 9
S5.3 Polarization dependence ..... 10
S5.4 Spectral Width ..... 11
S6 Fano resonance measurements ..... 14
S7 References ..... 15

# S1 Methods

All reagents were used as received from Sigma-Aldrich. Double Distilled Water (DDW) (18.3 $M\Omega cm^{-1}$) was used in all experiments.

## S1.1 Gold nanoparticles synthesis

The synthesis of the gold nanoparticles (NPs) was done following the method described by Cohen-Hoshen[1].

### S1.1.1 13 nm Gold NP Synthesis

Gold nanoparticles (NPs) with diameter of 13 nm were prepared using the Slot and Geuze method[2] with some modifications. A solution of 25 μL 1% Tannic Acid and 4 ml 1% $Na_3$citrate in 16 mL DDW was heated to 60 $^{\circ}$C and then added while vigorous stirring to a 60 $^{\circ}$C solution of 1 ml 1% $NaAuCl_4$ in 79 ml DDW. The mixed solution was then heated to boil for 10 min and then cooled to room temperature.

### S1.1.2 30 nm Gold NP Synthesis

3 ml of 13 nm gold NP solution is put in a 50 ml plastic falcon tube.

Add 48 ml 0.01% $NaAuCl_4$ + 2016 μl 40 mM hydroxylamine ($NH_2OH$) using the following scheme:

1. Repeat 15 times:
    a. 42 μl of 40 mM hydroxylamine ($NH_2OH$) is added under vigorous stirring.
    b. 1 ml of 0.01% $NaAuCl_4$ is added under stirring on vortex.
2. The NP solution is transferred to an Erlenmeyer.
3. Repeat 6 times:
    a. 210 μl of 40 mM hydroxylamine ($NH_2OH$) is added under vigorous stirring.
    b. 5 ml of 0.01% $NaAuCl_4$ is added under stirring on vortex.
4. 126 μl of 40 mM hydroxylamine ($NH_2OH$) is added under vigorous stirring.
5. 3 ml of 0.01% $NaAuCl_4$ is added under stirring on vortex.
6. Heat to boil; boil for 10 min (while stirring).
7. Cool to room temperature (no stirring).

### S1.1.3 55 nm Gold NP Synthesis

1. Put 21 ml of the 30 nm gold NP solution in an Erlenmeyer.
2. Add while stirring 10 ml 0.01% $NaAuCl_4$ + 420 μl 40 mM hydroxyl amine ($NH_2OH$).
3. Repeat step 2 until 145.5 ml of 0.01% $NaAuCl_4$ + 6111 μl of 40 mM hydroxyl amine ($NH_2OH$) were added.

The NPs were then capped by mercaptosuccinic-acid (MSA) ligands by adding 21 μl of ($10^{-2}$ M MSA in MeOH) to 6 ml of the NPs' solution, and waiting at room temperature for 3 hours.

Transmission Electron Microscopy (TEM) images of such NPs are shown in Figure S1:

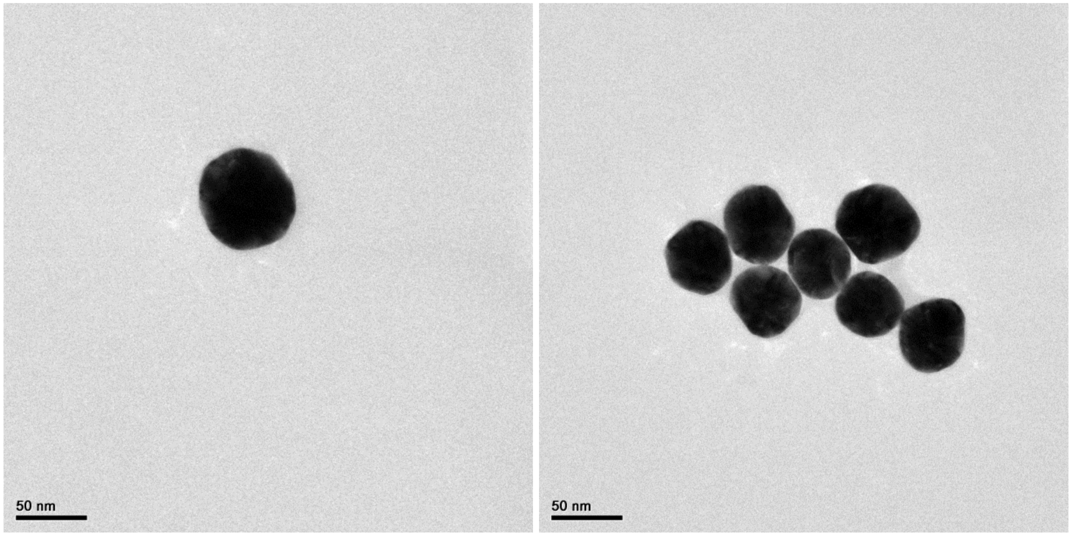


*Figure S1: TEM images of the nanoparticles*

## S1.2 Device fabrication and electrostatic trapping

Fabrication of the device, and electrostatic trapping of the nanoparticles, were done following the method described by Guttman[3] and Vardi[4]. Gold electrodes with a thickness of 25 nm and gap of 30 nm were fabricated on a heavily doped Si substrate, covered by 100 nm insulating $SiO_2$, using electron-beam (e-beam) lithography. A layer of 2 nm Nickel was used as an adhesion layer for the electrodes.

Nanoparticles (NPs) were connected to the electrodes using an electrostatic trapping method[5]. An alternating voltage of 1 V at 10 MHz was applied for 60 sec between the two electrodes, after covering them with a droplet of the NPs' solution (0.4 µl). The NPs are then trapped in the gap between the electrodes, where the electric field magnitude is larger.

Scanning Electron Microscopy (SEM) images of trapped NP of different devices are shown in Figure S2:

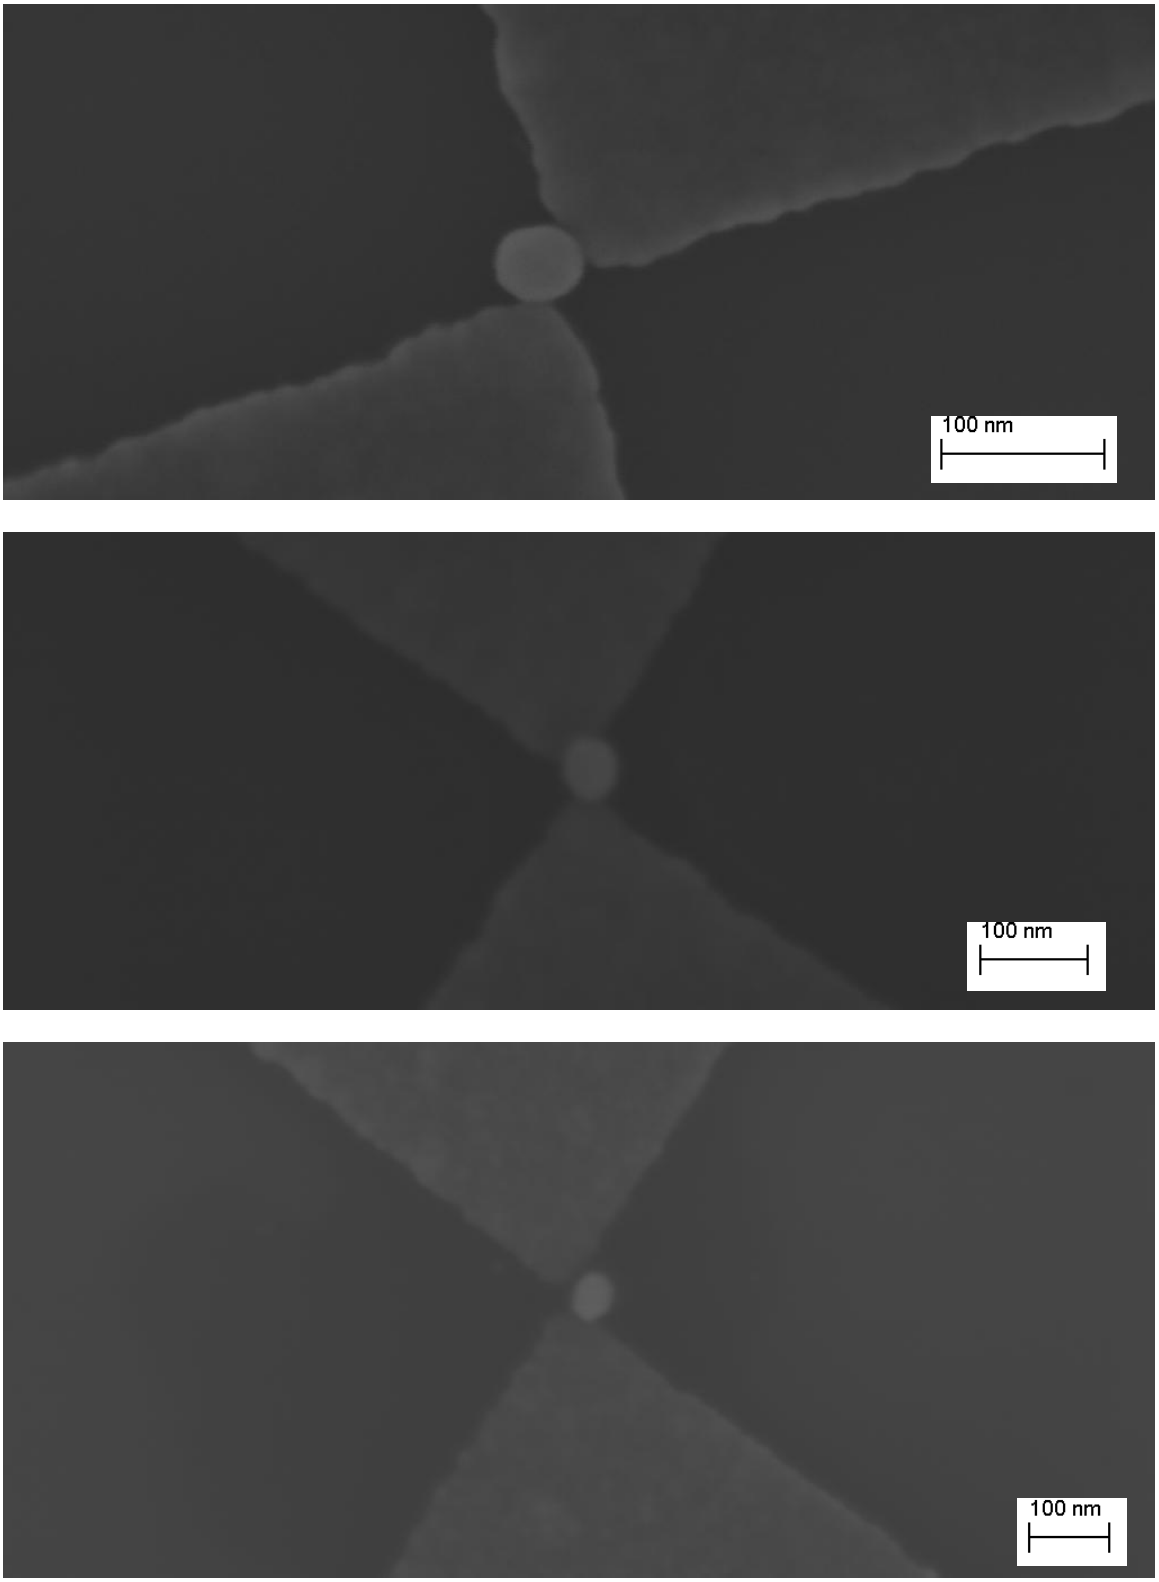


*Figure S2: Scanning Electron Microscopy (SEM) images of trapped nanoparticles in different devices*

## S2 Single dot simulation

The current through a single dot system can be written[6,7] as the difference between the forward and backward tunneling rates at each of the two tunnel barriers in the system:

$$I = |e| \sum_n P(n)[\gamma_i^+(n) - \gamma_i^-(n)]$$

Here, $e$ is the electron charge, $P(n)$ is the probability for finding the system with $n$ extra electrons in the NP, and $\gamma_i^{\pm}$ is the tunneling rate through the i'th barrier which is either in forward (+) or backward (-) direction.

The tunneling rate $\gamma_i$ is determined by the electrons' temperature T, the barrier conductivity $\mathrm{G}_i$, and the energy difference between the initial and final states of the system $\Delta\mathrm{E}_i$ (which is determined by the charging state $(n)$, the bias voltage $V_{SD}$, the back-gate voltage $V_G$ and the capacitances of the system) according to:

$$\gamma_i = \frac{G_i}{e^2} \frac{\Delta\mathrm{E}_i}{1 - Exp(-\Delta\mathrm{E}_i / k_B T)}$$

Using the Nelder-Mead simplex find method[8], we found the system's parameters (capacitances and two tunneling resistances) that best correspond to the measured results[3,4].

In Figure S3, we present the measured conductance spectra and the corresponding fits for several devices.

Device A:

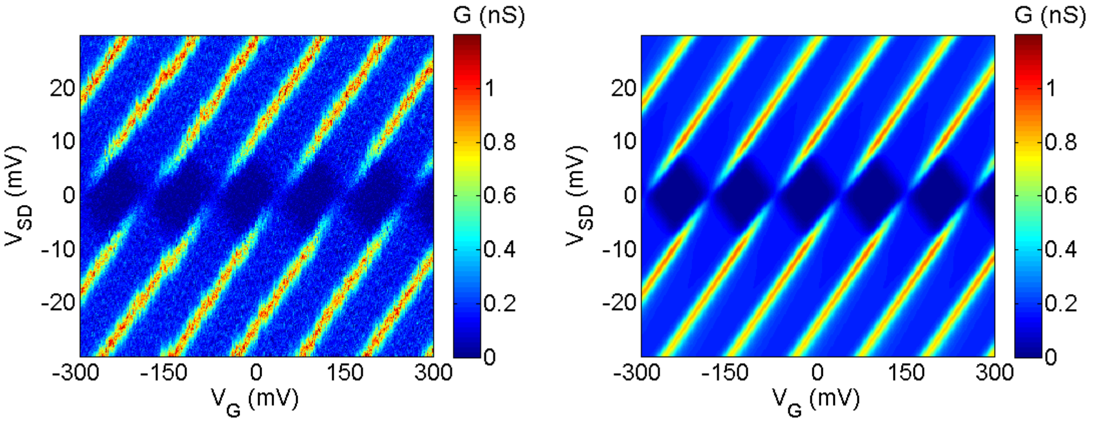


Device B:

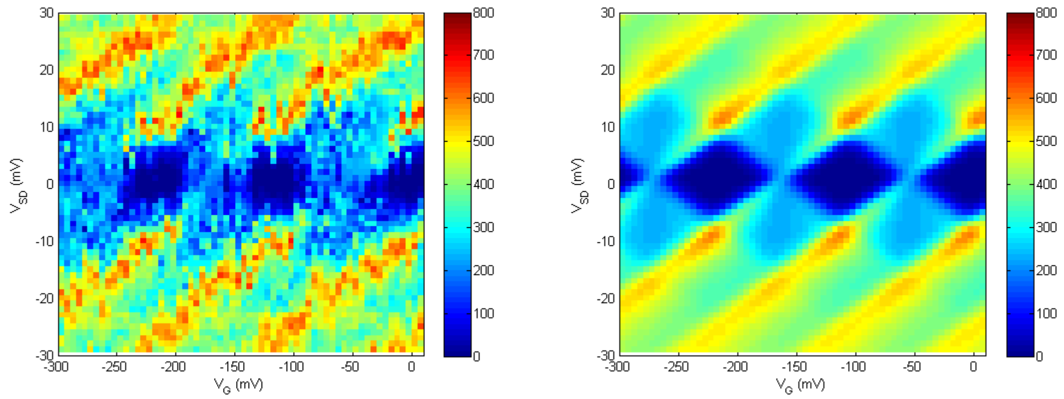


*Figure S3: Differential conductance measurements (left) and the corresponding simulations (right).*

## S2.1 Fit parameters

In Table S1 we show the fit parameters that were used to obtain the right panels in Figure S3. $C_j$ and $g_i$ are the capacitance (in aF) and conductance (in nS) between the NP and component i: L & R represent the left and right leads, and BG represents the back gate.

*Table S1: The fit parameters for Devices A and B*

| Device | $C_{BG}$ | $C_L$ | $C_R$ | $g_L$ | $g_R$ | $g_R/ g_L$ |
|---|---|---|---|---|---|---|
| A | 1.45 | 7.70 | 9.46 | 0.3 | 20.1 | 67 |
| B | 1.48 | 8.56 | 9.67 | 652 | 1641 | 2.5 |

The resulting charging energies are shown in Table S2.

*Table S2: The individual charging energies of the NPs (*in meV)

| Device | $E_C$ |
|---|---|
| A | 8.6 |
| B | 8.1 |

## S3 Symmetric and Asymmetric devices

Devices with high asymmetry in the conductance properties, such as device A in S3 above and the devices shown in Figure 3 in the main text, experience voltage division in which almost the entire applied voltage falls on a single tunnel junction. For example, for device A, where $g_R/g_L \approx 67$, more than 98% of the applied voltage $V_{SD}$ falls on the left barrier. Therefore, the emission spectrum measured has a cutoff energy, which is almost exactly $V_{SD}$.

Other devices, such as device B, which experience more symmetric voltage division between the two barriers, show emission spectra with a clear cutoff far from the applied $V_{SD}$. As discussed in the main text, symmetric devices experience large temporal fluctuations in the spectrum, and in particular in the cutoff energy.

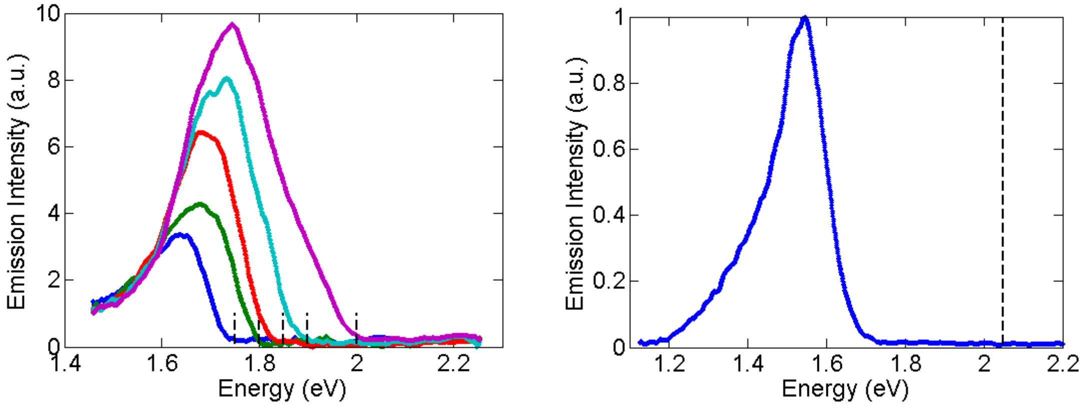


*Figure S4: Emission spectrum of device A (left) and B (right), measured with various $V_{SD}$ (marked with dashed lines on the figures). While at device A the energy cutoff equals $V_{SD}$, at device B a large gap is seen due to the more symmetrical voltage division between the two barriers.*

## S4 Extraction of plasmonic spectrum lineshape from total intensity measurement

In the main text we discuss the extraction of the plasmonic spectrum lineshape from a simple measurement of the total emitted intensity as a function of the applied voltage, P(V), and calculating its second derivative. We have demonstrated it on a device, as shown in Figure 3(a). Here we present the usage of this method on another device, revealing the extraction of its spectrum (Figure S5).

Notice that a direct measurement of the emitted spectrum from this device is shown in the main text in Figure 3(b-c). The spectrum extracted by the second derivative method (red line in Figure S5) corresponds very well to the direct measurement of the spectrum, as shown in Figure 3(c).

In addition, one can notice that the total intensity rises linearly once the cutoff voltage $V_{SD}$ moved across the plasmonic spectrum $g(\omega)$ (here, for $V_{SD}$>2V), with agreement with Eq. 2 in the main text.

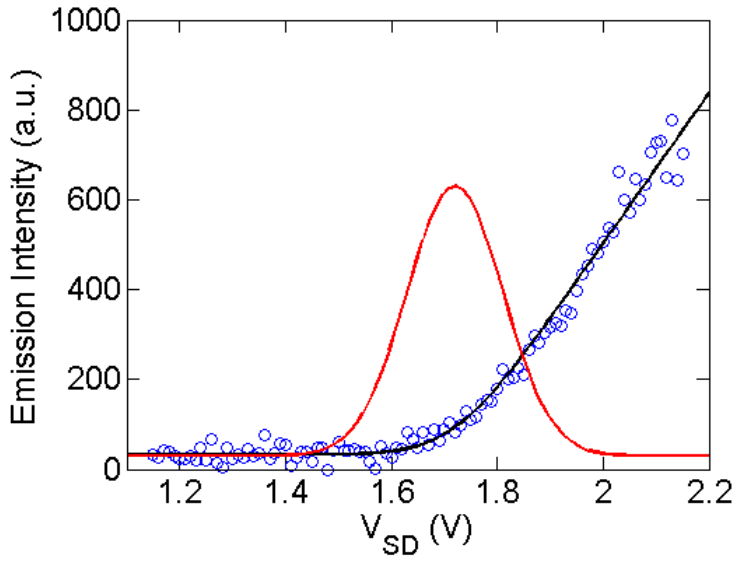


*Figure S5: Total intensity measurement of the light emission from a device (blue circles), and the extracted plasmonic spectra from the second derivate method (red solid line).*

# S5 FDTD Simulation

## S5.1 FDTD details

The scattering cross-sections calculations were done by commercial software "Lumerical FDTD Solutions". The electrodes were modeled by two flat, tapered gold slabs. Their tips were rounded with a 70 nm radius circles. The gap between the two electrodes was 30nm (edge to edge) and with-in it was placed a gold disk with a 30nm radius. The disk was positioned as such to have a 2 nm gap from both electrodes. The thickness of all objects was 25nm. For the dielectric functions of gold we used Johnson and Christy[9].

## S5.2 Insensitivity to electrodes design

We discussed in the main text the ability to control the Fano resonance energy and line-width by the nanoparticle geometry (Figure 4(c)). Here we show that the resonance is relatively insensitive to the details of the electrodes design: when changing the angle of the bow-tie electrodes we find that the Fano dip remains at approximately the same spectral position.

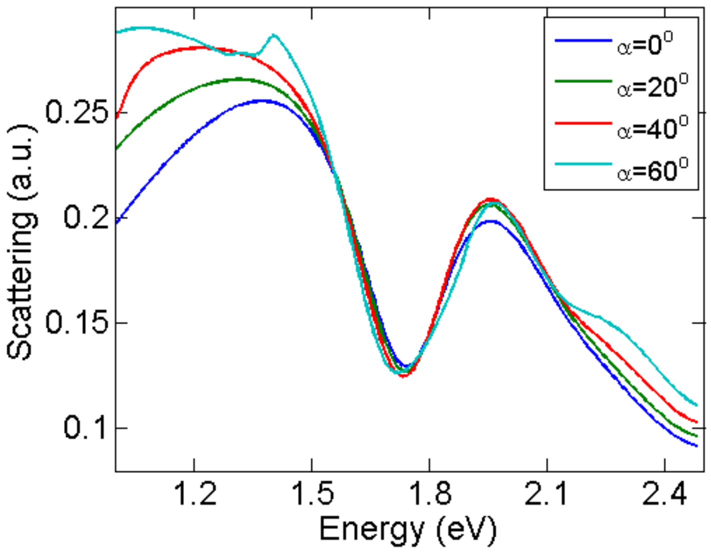


*Figure S6: FDTD simulation of the scattering cross-section of bow-tie electrodes and a trapped circular nanoparticle. $\alpha$ is the flare angle of the bow-tie structure.*

## S5.3 Polarization dependence

The Fano spectral shape is obtained when the excitation is in the X-axis direction (axes as in the sketch at the top of Figure 4(b) in the main text).

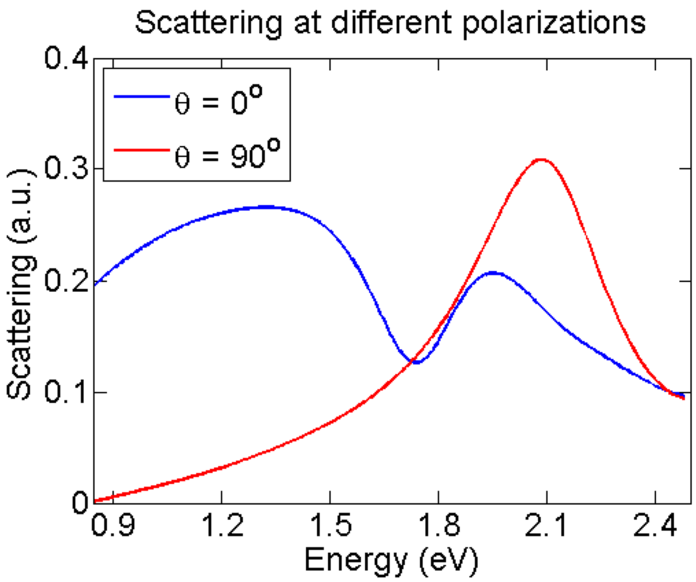


*Figure S7: FDTD simulation of the scattering cross-section of bow-tie electrodes and a trapped circular nanoparticle, at different excitation polarization (the angle θ is measured with respect to the X-axis, as in the sketch at the top of Figure 4(b) in the main text).*

## S5.4 Spectral Width

It is seen that the experimental spectral features (scattering and emission – Figures 3 and 4(a) in the main text) are narrower than those obtained in the simulation (Figure 4(b)). This could be explained by the fact that our electrodes were formed by evaporation, consisting of large grains (typically tens of nanometers).

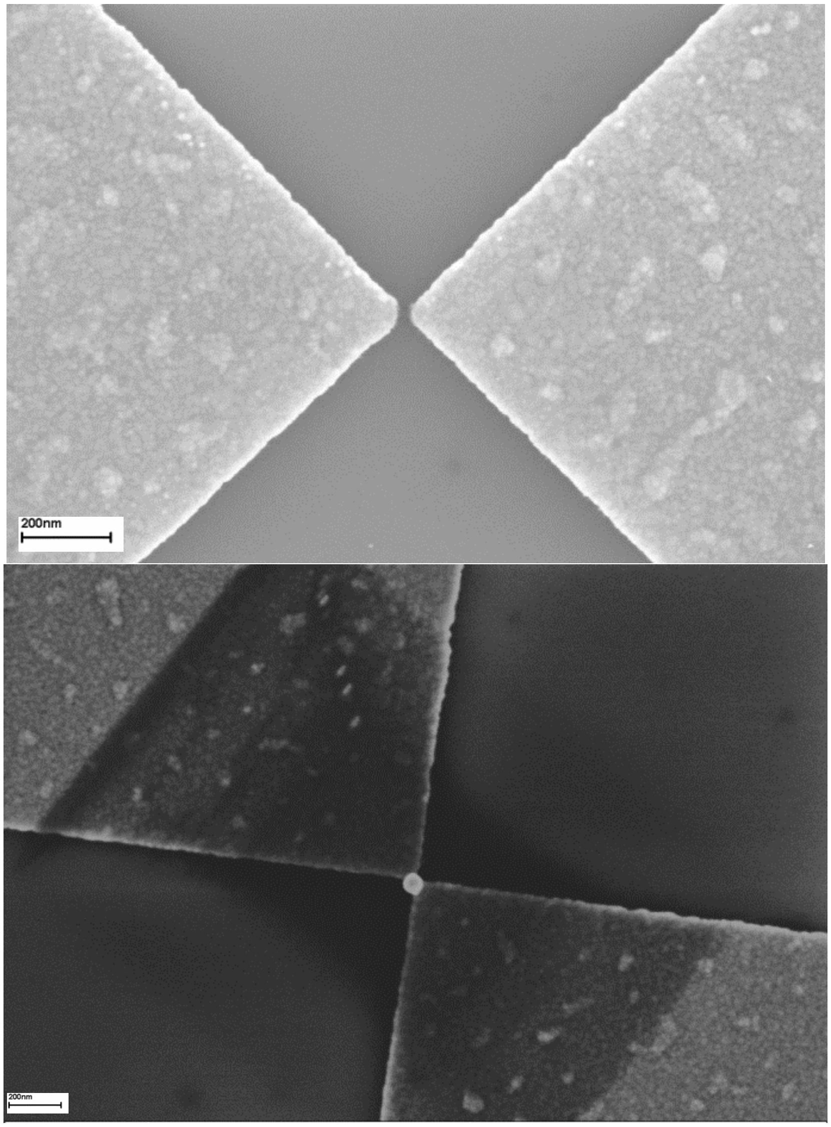


*Figure S8: Scanning-Electron Microscope (SEM) images of typical devices, show the graininess of the evaporated electrodes.*

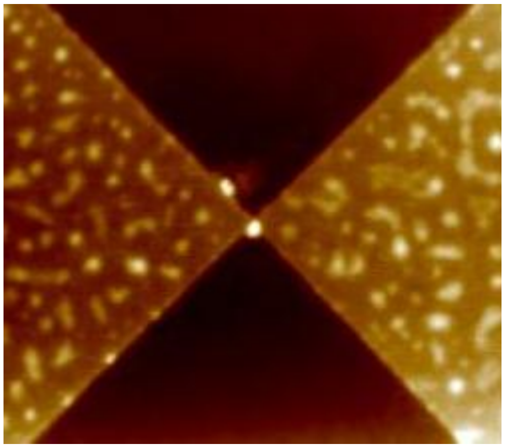

*Figure S9: Atomic-Force Microscope (AFM) image of a typical device, shows the graininess of the evaporated electrodes.*

It is well known that the plasmonic spectrum of such grainy films is much narrower than that of “ideal” continuous metal layers, which were assumed in our calculation[10–13].

We also notice that the observed Fano resonance is significantly narrower than the one showed in Figure 4(b). We find that the width of the dip is very sensitive to the size of the tunnel gap between the NP and the electrodes. This is demonstrated in the figure below, which shows the evolution of the Fano dip as the tunnel junction width is changed from narrow (cyan) to wide (red). We note that these simulations were conducted for a disk. The Fano dip of a spherical nanoparticle would be as having an effective large mean gap, i.e. – narrower dip.

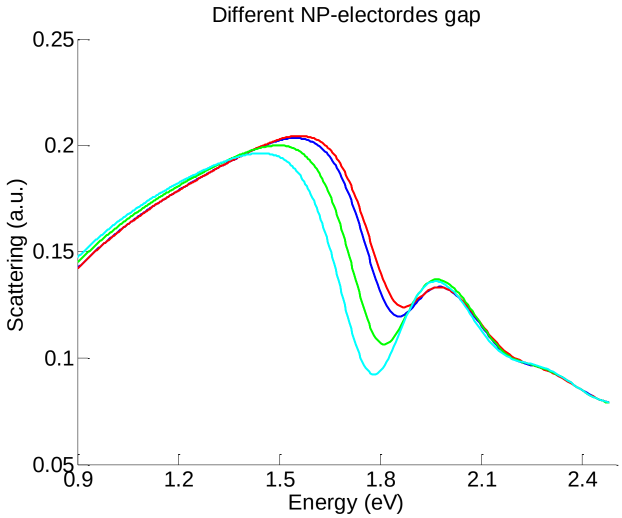


*Figure S10: FDTD calculation of the scattering spectrum with different NP-electrodes gap size, from narrow (cyan) to wide (red).*

Another source of narrowing of the Fano dip can be attributed to deviation from spherical symmetry of the NP. It is evident in Figure 4c of the paper that as the eccentricity of nanoparticle is increased the Fano dip becomes narrower: the peak to dip energy difference decreases by approximately a factor of two as the spherical disk becomes a narrow ellipse.

Taking these factors into account, namely – a more realistic NP structure and a wide effective gap, we can obtain a Fano dip, which is similar in width to the one obtained experimentally.

## S6 Fano resonance measurements

Note different measurements of the Fano resonance spectral lineshape.

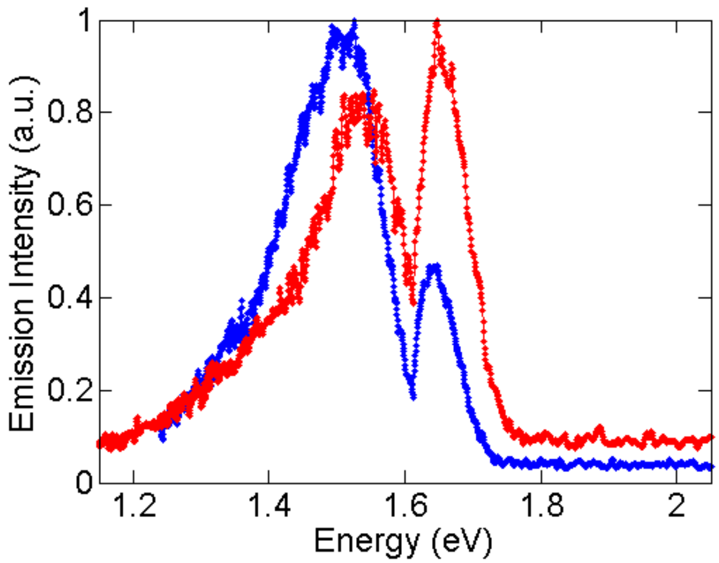


*Figure S10: Several measurements of Fano resonance spectrum, normalized.*

## S7 References


(1) Cohen-Hoshen, E.; Bryant, G. W.; Pinkas, I.; Sperling, J.; Bar-Joseph, I. *Nano Lett.* **2012**, *12*, 4260–4264.

(2) Slot, J. W.; Geuze, H. J. *Eur. J. Cell Biol.* **1985**, *38*, 87–93.

(3) Guttman, A.; Mahalu, D.; Sperling, J.; Cohen-Hoshen, E.; Bar-Joseph, I. *Appl. Phys. Lett.* **2011**, *99*, 063113.

(4) Vardi, Y.; Guttman, A.; Bar-Joseph, I. *Nano Lett.* **2014**, *14*, 2794–2799.

(5) Bezryadin, A.; Dekker, C.; Schmid, G. *Appl. Phys. Lett.* **1997**, *71*, 1273.

(6) Grabert, H.; Devoret, M. H. *Single Charge Tunneling: Coulomb Blockade Phenomena in Nanostructures:[Proceedings of the NATO Advanced Study Institute on Single Charge Tunneling, Held March 5-15, 1991, in Les Houches, France]*; Grabert, H.; Devoret, M. H., Eds.; Plenum Press: New York, 1992.

(7) Beenakker, C. W. J. *Phys. Rev. B* **1991**, *44*, 1646–1656.

(8) Nelder, J. A.; Mead, R. *Comput. J.* **1965**, *7*, 308–313.

(9) Johnson, P. B.; Christy, R. W. *Phys. Rev. B* **1972**, *6*, 4370–4379.

(10) Geddes, C. D. *Reviews in Plasmonics 2010*; Geddes, C. D., Ed.; Reviews in Plasmonics; Springer New York: New York, NY, 2012; Vol. 2010.

(11) Szunerits, S.; Praig, V. G.; Manesse, M.; Boukherroub, R. *Nanotechnology* **2008**, *19*, 195712.

(12) Olmon, R. L.; Slovick, B.; Johnson, T. W.; Shelton, D.; Oh, S.-H.; Boreman, G. D.; Raschke, M. B. *Phys. Rev. B* **2012**, *86*, 235147.

(13) Sun, H.; Yu, M.; Wang, G.; Sun, X.; Lian, J. *J. Phys. Chem. C* **2012**, *116*, 9000–9008.
